# Supplementary material for: PAC Statistical Model Checking of Mean Payoff in Discrete- and Continuous-Time MDP
Source: arXiv:2206.01465 source file (2022-06-03)
Supplement: Supplementary file 2 [file appendix_new_ctmdp_results.tex]

\section{New CTMDP Results}
\label{app:newCtmdpResults}

\begin{table}[]
\centering
\scalebox{0.9}{
\begin{tabular}{|l|l|l|llll|llll|}
\hline
\multicolumn{1}{|c|}{\multirow{2}{*}{Benchmarks}} &
  \multicolumn{1}{c|}{\multirow{2}{*}{\begin{tabular}[c]{@{}c@{}}Number\\ of states\end{tabular}}} &
  \multicolumn{1}{c|}{\multirow{2}{*}{Value}} &
  \multicolumn{4}{c|}{Blackbox} &
  \multicolumn{4}{c|}{\begin{tabular}[c]{@{}c@{}}Blackbox with \\ greybox update equations\end{tabular}} \\ \cline{4-11} 
\multicolumn{1}{|c|}{} &
  \multicolumn{1}{c|}{} &
  \multicolumn{1}{c|}{} &
  \multicolumn{1}{c|}{\begin{tabular}[c]{@{}c@{}}States\\ explored\end{tabular}} &
  \multicolumn{1}{c|}{\begin{tabular}[c]{@{}c@{}}lower\\ bound\end{tabular}} &
  \multicolumn{1}{c|}{\begin{tabular}[c]{@{}c@{}}upper\\ bound\end{tabular}} &
  \multicolumn{1}{c|}{\begin{tabular}[c]{@{}c@{}}Time\\ (s)\end{tabular}} &
  \multicolumn{1}{c|}{\begin{tabular}[c]{@{}c@{}}States\\ explored\end{tabular}} &
  \multicolumn{1}{c|}{\begin{tabular}[c]{@{}c@{}}lower\\ bound\end{tabular}} &
  \multicolumn{1}{c|}{\begin{tabular}[c]{@{}c@{}}upper\\ bound\end{tabular}} &
  \multicolumn{1}{c|}{\begin{tabular}[c]{@{}c@{}}Time\\ (s)\end{tabular}} \\ \hline
DynamicPM &
  816 &
  1.0 &
  \multicolumn{1}{l|}{816} &
  \multicolumn{1}{l|}{0.436} &
  \multicolumn{1}{l|}{1.0} &
  TO &
  \multicolumn{1}{l|}{816} &
  \multicolumn{1}{l|}{0.998} &
  \multicolumn{1}{l|}{1.0} &
  37.68 \\ \hline
ErlangStages &
  508 &
  1.0 &
  \multicolumn{1}{l|}{508} &
  \multicolumn{1}{l|}{0.962} &
  \multicolumn{1}{l|}{1.0} &
  TO &
  \multicolumn{1}{l|}{508} &
  \multicolumn{1}{l|}{0.999} &
  \multicolumn{1}{l|}{1.0} &
  8.118 \\ \hline
PollingSystem1 &
  16 &
  0.922 &
  \multicolumn{1}{l|}{16} &
  \multicolumn{1}{l|}{0.811} &
  \multicolumn{1}{l|}{0.937} &
  TO &
  \multicolumn{1}{l|}{16} &
  \multicolumn{1}{l|}{0.816} &
  \multicolumn{1}{l|}{0.937} &
  TO \\ \hline
PollingSystem2 &
  348 &
  0.999 &
  \multicolumn{1}{l|}{348} &
  \multicolumn{1}{l|}{0.637} &
  \multicolumn{1}{l|}{0.999} &
  TO &
  \multicolumn{1}{l|}{348} &
  \multicolumn{1}{l|}{0.998} &
  \multicolumn{1}{l|}{0.999} &
  21.893 \\ \hline
PollingSystem3 &
  1002 &
  0.999 &
  \multicolumn{1}{l|}{1002} &
  \multicolumn{1}{l|}{0.232} &
  \multicolumn{1}{l|}{1.0} &
  TO &
  \multicolumn{1}{l|}{1002} &
  \multicolumn{1}{l|}{0.99} &
  \multicolumn{1}{l|}{1.0} &
  864.05 \\ \hline
QueuingSystem &
  266 &
  0.8783 &
  \multicolumn{1}{l|}{266} &
  \multicolumn{1}{l|}{0.703} &
  \multicolumn{1}{l|}{0.906} &
  TO &
  \multicolumn{1}{l|}{266} &
  \multicolumn{1}{l|}{0.865} &
  \multicolumn{1}{l|}{0.886} &
  TO \\ \hline
SJS1 &
  17 &
  1.0 &
  \multicolumn{1}{l|}{17} &
  \multicolumn{1}{l|}{0.999} &
  \multicolumn{1}{l|}{1.0} &
  133.96 &
  \multicolumn{1}{l|}{17} &
  \multicolumn{1}{l|}{0.997} &
  \multicolumn{1}{l|}{1.0} &
  1.05 \\ \hline
SJS2 &
  7393 &
  0.999 &
  \multicolumn{1}{l|}{7341} &
  \multicolumn{1}{l|}{0.02} &
  \multicolumn{1}{l|}{1.0} &
  TO &
  \multicolumn{1}{l|}{7268} &
  \multicolumn{1}{l|}{0.936} &
  \multicolumn{1}{l|}{1.0} &
  TO \\ \hline
SJS3 &
  433 &
  1.0 &
  \multicolumn{1}{l|}{433} &
  \multicolumn{1}{l|}{0.919} &
  \multicolumn{1}{l|}{1.0} &
  TO &
  \multicolumn{1}{l|}{432} &
  \multicolumn{1}{l|}{0.999} &
  \multicolumn{1}{l|}{0.999} &
  5.3814 \\ \hline
toy &
  12 &
  1.0 &
  \multicolumn{1}{l|}{12} &
  \multicolumn{1}{l|}{0.99} &
  \multicolumn{1}{l|}{1.0} &
  5.6 &
  \multicolumn{1}{l|}{12} &
  \multicolumn{1}{l|}{0.999} &
  \multicolumn{1}{l|}{1.0} &
  1.112 \\ \hline
\end{tabular}
}
\caption{Results on CTMDP benchmarks}
\label{tab:newCtmdpResults}
\end{table}
